# Supplementary material for: Cosmology using Strong Gravitational Lensing
Source: arXiv:2405.03397 source file (2024-05-06)
Supplement: Supplementary file 1 [file AppendixTemplate.tex]

% Appendix Template

\chapter{Appendix Title Here} % Main appendix title

\label{AppendixX} % Change X to a consecutive letter; for referencing this appendix elsewhere, use \ref{AppendixX}

Write your Appendix content here.
